# Supplementary material for: Indecision Modeling
Source: arXiv:2012.08485 source file (2021-03-12)
Supplement: Supplementary file 1 [file appendix_score_based_indecision.tex]

In this section we re-formalize each of the indecision models introduced in the previous section using \emph{score functions}.
The score-based decision models in this section are defined using two functions: $S:\mathcal I \times \mathcal I \rightarrow \mathbb R$ is the score function for strict preference responses (i.e., score $S(i, j)$ is the score for response $i\succ j$), and $F :\mathcal I \times \mathcal I \rightarrow \mathbb R$ is the score function for indecision responses (i.e., $F(i, j)$ is the score for response $i \sim j$).

Using these scoring functions, the \emph{score-based response model} is
$$ 
R(i, j; S,F) \equiv \begin{cases}
1 & \text{if}\,\, S(i, j) \geq S(j, i) \,\,\text{and}\,\, S(i,j) > F(i, j)\\
    2 &\text{if}\,\,  S(i, j) < S(j, i) \,\,\text{and}\,\, S(j, i) > F(i, j) \\
0 &\text{otherwise} \\
\end{cases}
$$
In other words, the agent responds according to which score function is maximal, where ties are broken first in favor of response $0$ and then $1$.
Next we propose score functions which yield score-based response models equivalent to each of the indecision models from the previous section.

\subsection{Difference-Based Scoring Functions}
\paragraph{Min-Difference}
\begin{equation*}
    \begin{array}{rl}
         S^D_-(i, j) &\equiv u(i) - u(j) \\
         F^D_-(i, j) &\equiv \lambda 
    \end{array}
\end{equation*}

\begin{lem}
The score-based decision function $R(S^S_-, F^S_-;\cdot, \cdot)$ is equivalent to $R^S_-(\cdot, \cdot)$.
\end{lem}

\DCM{move to appendix:} 

\begin{proof}
We show that for both strict and indecision responses, decision rules $R^D_-(i,j)$ and $R(i,j;S^D_-, F^D_-)$ result in equivalent constraints on $u(i)$, $u(j)$, and $\lambda$.
\paragraph{Strict responses: $i \succ j$}
The following two statements are equivalent, for $\lambda>0$:
$$
u(i) > u(j) + \lambda \iff 
\begin{array}{l} 
u(i) \geq u(j) \\
\land u(i) - u(j) > \lambda
\end{array} 
$$
where the left side is equivalent to the conditions for $R^D_-(i,j)$ if $i \succ j$, and the right side is equivalent to the conditions for $R(i,j;S^D_-, F^D_-)$ if $i \succ j$.

Note that a similar reasoning applies to $i \prec j$.

\paragraph{Indecision responses: $i \sim j$}
The following two statements are equivalent, for $\lambda>0$:
$$
|u(i) - u(j)| \leq \lambda \iff 
\begin{array}{l} 
u(i) - u(j) \leq \lambda \\
\land u(j) - u(i) \leq \lambda
\end{array} 
$$
\end{proof}

\paragraph{Max-Difference}

\begin{equation*}
    \begin{array}{rl}
         S^D_+(i, j) &\equiv  u(i) - u(j)  \\
         F^D_+(i, j) &\equiv 2|u(i) - u(j)| - \lambda
    \end{array}
\end{equation*}

\begin{lem}
The score-based decision function $R(S^S_+, F^S_+;\cdot, \cdot)$ is equivalent to $R^S_+(\cdot, \cdot)$.
\end{lem}

\DCM{move to appendix:}

\begin{proof}
We show that for both strict and indecision responses, decision rules $R^D_+(i,j)$ and $R(i,j;S^D_+, F^D_+)$ result in equivalent assumptions on $u(i)$, $u(j)$, and $\lambda$.
\paragraph{Strict responses: $i \succ j$}
The following two statements are equivalent, for $\lambda>0$:
$$
\begin{array}{l} 
u(i) \geq u(j) \\
\land u(i) - u(j) <  \lambda 
\end{array} 
\iff 
\begin{array}{l} 
u(i) \geq u(j) \\
\land u(i) - u(j) > 2 | u(i) - u(j)| - \lambda  \\
\end{array} 
$$
since the right side reduces to $u(i) - u(j) < \lambda$.
As before, the left side is equivalent to the conditions for $R^D_+(i,j)$ if $i \succ j$, and the right side is equivalent to the conditions for $R(i,j;S^D_+, F^D_+)$ if $i \succ j$.
Note that similar reasoning applies to $i \prec j$.

\paragraph{Indecision responses: $i \sim j$}
The following two statements are equivalent, for $\lambda>0$:
$$
|u(i) - u(j)| \geq \lambda \iff 
\begin{array}{l} 
2 |u(i) - u(j)| - \lambda \geq u(i) - u(j) \\
\land 2 |u(i) - u(j)| - \lambda \geq u(j) - u(i)
\end{array} 
$$
\end{proof}

\paragraph{Min-Likability}
\begin{equation*}
    \begin{array}{rl}
         S^L_-(i, j) &\equiv u(i)  \\
         F^L_-(i, j) &\equiv \lambda
    \end{array}
\end{equation*}
\begin{lem}
The score-based decision function $R(S^L_-, F^L_-;\cdot, \cdot)$ is equivalent to $R^L_-(\cdot, \cdot)$.
\end{lem}
\begin{proof}
We show that for both strict and indecision responses, decision rules $R^L_-(i,j)$ and $R(i,j;S^L_-, F^L_-)$ result in equivalent assumptions on $u(i)$, $u(j)$, and $\lambda$.
\paragraph{Strict responses: $i \succ j$}
Note that both decision models require the same inequalities, reproduced here for clarity:
\begin{align*}
u(i)  \geq u(j) \,\,\,\land \,\,\,u(i) > \lambda 
\end{align*}
 and as before, similar reasoning applies to $i \prec j$.

\paragraph{Indecision responses: $i \sim j$}
As before, both decision models require the same inequalities for response $i \sim j$, reproduced here for clarity:
$$u(i) \leq \lambda \,\,\, \land \,\,\, u(j) \leq \lambda $$
\end{proof}

\paragraph{Max-Likability}
\begin{equation*}
    \begin{array}{rl}
         S^L_+(i, j) &\equiv  u(i) \\
         F^L_+(i, j) &\equiv 2 \min\{u(i),u(j)\} - \lambda
    \end{array}
\end{equation*}
\begin{lem}
The score-based decision function $R(S^S_+, F^S_+;\cdot, \cdot)$ is equivalent to $R^S_+(\cdot, \cdot)$.
\end{lem}

\DCM{move to appendix: }

\begin{proof}
We show that for both strict and indecision responses, decision rules $R^L_+(i,j)$ and $R(i,j;S^L_+, F^L_+)$ result in equivalent assumptions on $u(i)$, $u(j)$, and $\lambda$.
\paragraph{Strict responses: $i \succ j$}
The following two statements are equivalent, for $\lambda>0$:
$$
\begin{array}{l} 
u(i) \geq u(j) \\
\land u(j) < \lambda
\end{array} 
\iff 
\begin{array}{l} 
u(i) \geq u(j) \\
\land u(i) >  2\min\{u(i), u(j)\} - \lambda \\
\end{array} 
$$
since the right side reduces to $\lambda > 0$.
As before, the left side is equivalent to the conditions for $R^D_+(i,j)$ if $i \succ j$, and the right side is equivalent to the conditions for $R(i,j;S^D_+, F^D_+)$ if $i \succ j$.
Note that similar reasoning applies to $i \prec j$.

\paragraph{Indecision responses: $i \sim j$}
The following two statements are equivalent, for $\lambda>0$:
$$
|u(i) - u(j)| \geq \lambda \iff 
\begin{array}{l} 
2 |u(i) - u(j)| - \lambda \geq u(i) - u(j) \\
\land 2 |u(i) - u(j)| - \lambda \geq u(j) - u(i)
\end{array} 
$$
\end{proof}

\paragraph{Dominance}
\begin{align*}
    S^M(i,j) &\equiv \min_{n \in [N]}\left(u_n(i) - u_n(j)\right) \\
    F^M(i, j) &\equiv \lambda 
\end{align*}
\begin{lem}
The score-based decision function $R(S^M, F^M;\cdot, \cdot)$ is equivalent to $R^M(\cdot, \cdot)$.
\end{lem}

\DCM{move to appendix: }

\begin{proof}
We show that for both strict and indecision responses, decision rules $R^M(i,j)$ and $R(i,j;S^M, F^M)$ result in equivalent assumptions on $u(i)$, $u(j)$, and $\lambda$.
\paragraph{Strict responses: $i \succ j$}
The following two statements are equivalent, for $\lambda>0$:
\begin{equation*}
\begin{array}{c}
u_k(i) \geq u_k(j) + \lambda \\ \forall k=1, \dots, K
\end{array}
{\tiny\iff}
\begin{array}{c}
\min\limits_{n \in [N]}\left(u_n(i) - u_n(j)\right)\geq \lambda \\
\land \min\limits_{n \in [N]}\left(u_n(i) - u_n(j)\right) > \min\limits_{n \in [N]}\left(u_n(j) - u_n(i)\right)
\end{array}
\end{equation*}
As before, the left side is equivalent to the conditions for $R^M(i,j)$ if $i \succ j$, and the right side is equivalent to the conditions for $R(i,j;S^M, F^M)$ if $i \succ j$.
Similar reasoning holds for strict response $i \prec j$.

\paragraph{Indecision responses: $i \sim j$}
The following two statements are equivalent, for $\lambda>0$:
\begin{equation*}
\begin{array}{c}
\exists n \in [N]: u_n(i) < u_n(j) + \lambda \\
\lor u_n(j) < u_n(i) + \lambda 
\end{array}
\iff\\
\begin{array}{c}
\lambda > \min\limits_{n \in [N]}\left(u_n(i) - u_n(j)\right)\\
\land \lambda > \min\limits_{n \in [N]}\left(u_n(j) - u_n(i)\right)
\end{array}
\end{equation*}
\end{proof}

The score-based indecision models in this section are equivalent to the utility-based decision models in Section~\ref{sec:indecision-models}. 
However both sets of models suffer from a similar problem: they assume that agents respond \emph{consistently} according to a utility function $u(\cdot)$ and threshold $\lambda$.
In reality, agents may respond inconsistently (according to one of our indecision models), or they may respond according to a \emph{different} indecision model--which may or may not be similar to one of our proposed model classes.
Both of these effects can be approximated by random ``noise'' in agent responses~\cite{???}.
Furthermore, assuming noisy responses yields a convenient probabilistic formulation for each indecision model; this is the focus of the next section.
