# Supplementary material for: Indecision Modeling
Source: arXiv:2012.08485 source file (2021-03-12)
Supplement: Supplementary file 2 [file appendix_results.tex]

\section{Model-Fitting Results}\label{app:model-results}

\begin{table*}
\caption{
Training and testing LL for each model. 
%
%
% The number of participants for which each model has the largest test log-likelihood (\#1st), second-largest test LL (\#2nd), and third-largest (\#3rd) are given for each model, and the median training and test LL over all participants.
}
\begin{tabular}{@{}lllllllllllll@{}}
\toprule
\multirow{3}{*}{\textbf{Model Name}} & \multicolumn{4}{c}{\textbf{20 Training Voters}}                    & \multicolumn{4}{c}{\textbf{50 Training Voters}}                    & \multicolumn{4}{c}{\textbf{100 Training Voters}}                   \\
                         \cmidrule(lr){2-5}  \cmidrule(lr){6-9}
                         \cmidrule(lr){10-13}
                        & \multirow{2}{*}{Train} & \multicolumn{3}{c}{Test (by voter type)}                          & \multirow{2}{*}{Train} & \multicolumn{3}{c}{Test (by voter type)}                          & \multirow{2}{*}{Train} & \multicolumn{3}{c}{Test (by voter type)}                          \\
                        \cmidrule(lr){3-5}
                        \cmidrule(lr){7-9}
                         \cmidrule(lr){11-13}
  &       & Train & Test    & All      &       & Train & Test     & All      &       & Train  & Test     & All      \\
  \midrule
  Mixture Models \\
$k=2$-\minD{}         & -0.90 & -0.88           & -0.89          & \textbf{-0.89} & -0.90 & \textbf{-0.88}  & \textbf{-0.87} & \textbf{-0.87} & -0.87 & -0.87           & -0.88          & -0.88          \\
$k=2$-\texttt{Mixture}            & -0.87 & \textbf{-0.86}  & -0.93          & -0.93          & -0.90 & \textbf{-0.88}  & -0.88          & -0.88          & -0.87 & -0.87           & -0.89          & -0.88          \\
\texttt{VoterMixture} & -0.92 & -0.90           & -0.97          & -0.96          & -0.96 & -0.95           & -0.95          & -0.95          & -0.93 & -0.93           & -0.94          & -0.94          \\
\midrule
Indecision Models \\
\minD{}              & -0.92 & -0.90           & \textbf{-0.90} & -0.90          & -0.90 & \textbf{-0.88}  & \textbf{-0.87} & \textbf{-0.87} & -0.87 & -0.87           & -0.88          & -0.87          \\
\maxD{}               & -0.95 & -0.90           & -0.96          & -0.96          & -1.00 & -0.97           & -0.95          & -0.95          & -0.96 & -0.95           & -0.95          & -0.95          \\
\maxL{}             & -0.87 & \textbf{-0.86}  & -0.93          & -0.93          & -0.95 & -0.93           & -0.94          & -0.94          & -0.94 & -0.94           & -0.95          & -0.94          \\
\minL{}               & -0.96 & -0.95           & -1.01          & -1.01          & -1.00 & -0.98           & -0.99          & -0.98          & -0.98 & -0.98           & -0.99          & -0.99          \\
\dom{}                   & -1.08 & -1.07           & -1.06          & -1.06          & -1.06 & -1.06           & -1.06          & -1.06          & -1.05 & -1.05           & -1.06          & -1.06          \\
\midrule
Baseline Models \\
\texttt{MLP}         & -0.40 & -1.55           & -1.72          & -1.70          & -0.59 & -0.99           & -1.17          & -1.11          & -0.71 & \textbf{-0.76}  & \textbf{-0.86} & \textbf{-0.77} \\
\flipLogit{}           & -0.91 & -0.88           & -0.95          & -0.95          & -0.96 & -0.94           & -0.93          & -0.93          & -0.93 & -0.93           & -0.94          & -0.94          \\
\texttt{NaiveRand}             & -1.03 & -1.00           & -1.09          & -1.08          & -1.08 & -1.07           & -1.07          & -1.07          & -1.07 & -1.07           & -1.07          & -1.07          \\
\texttt{UniformRand}           & -1.10 & -1.10           & -1.10          & -1.10          & -1.10 & -1.10           & -1.10          & -1.10          & -1.10 & -1.10           & -1.10          & -1.10          \\
\bottomrule
\end{tabular}
\end{table*}
